# Supplementary material for: Optimal Voltage Phasor Regulation for Switching Actions in Unbalanced Distribution Systems
Source: arXiv:1804.02080 source file (2019-06-26)
Supplement: Supplementary file 1 [file appendix.tex]

\section*{Appendix}
\label{sec:appendix}

\emph{Extension of Semidefinite OPF of} \cite{dall2013distributed}: We start by rewriting the matrix variable $\mathbf{V} = \mathbf{v} \mathbf{v}^{\mathcal{H}}$, where $\mathbf{v} = {\left[ \mathbf{V}_{0}^{T} , \qq \mathbf{V}_{1}^{T} , \qq \ldots \qq \mathbf{V}_{N}^{T} \right]}^{T}$ and $\mathbf{V}_{n} = {\left[ V_{n}^{a} , \qq V_{n}^{b} , \qq V_{n}^{c} \right]}^{T}$. The squared voltage magnitude of the phasor on phase $\phi$ at node $n$ is XXXXX

Now, consider an off-diagonal entry of $\mathbf{V}$, $\mathbf{V}_{mn}^{\phi} = V_{m}^{\phi} {\left( V_{n}^{\phi} \right)}^{*}$, corresponding to the product of the voltage phasor of phase $\phi$ at node $m$, and the complex conjugate of the voltage phasor of phase $\phi$ at node n:
\begin{equation}
	V_{m}^{\phi} {\left( V_{n}^{\phi} \right)}^{*} = \Tr \left( \Phi_{V,mn}^{\phi} \mathbf{V} \right) \qq .
\end{equation}

\noindent where $\Phi_{V,mn}^{\phi} = \overline{e}_{n}^{\phi} \left( \overline{e}_{m}^{\phi} \right)^{T}$

\noindent Here, we express this term in polar form, where we define $\theta_{mn}^{\phi} = \theta_{m}^{\phi} - \theta_{n}^{\phi}$:
\begin{equation}
% 	\mathbf{V}_{mn}^{\phi}
%     =
    V_{m}^{\phi} {\left( V_{n}^{\phi} \right)}^{*}
    =
    \left| V_{m}^{\phi} \right| \left| V_{n}^{\phi} \right| \angle \left( \theta_{m}^{\phi} - \theta_{n}^{\phi} \right)
    =
    \left| V_{m}^{\phi} \right| \left| V_{n}^{\phi} \right| \angle \theta_{mn}^{\phi} \qq .
    \label{VnV0polar}
\end{equation}

% \begin{equation}
% 	V_{n}^{\phi} \left( V_{0}^{\phi} \right)^{*} = \left| V_{n}^{\phi} \right| \left| V_{0}^{\phi} \right| \left[ \cos \left( \theta_{n}^{\phi} - \theta_{0}^{\phi} \right) + j \sin \left( \theta_{n}^{\phi} - \theta_{0}^{\phi} \right) \right] \label{VnV0rect} 
% \end{equation}

\noindent Using Euler's rule, we write the the real and imaginary parts of $\mathbf{V}_{mn}^{\phi}$ in terms of the tangent of $\theta_{mn}^{\phi}$:
% \begin{equation}
% 	\tan \left( \theta_{n}^{\phi} - \theta_{0}^{\phi} \right)
% %     =
% %     \frac{\sin \left( \theta_{n}^{\phi} - \theta_{0}^{\phi} \right)}{\cos \left( \theta_{n}^{\phi} - \theta_{0}^{\phi} \right)}
%     =
%     \frac{\Im \left\{ V_{n}^{\phi} \left( V_{0}^{\phi} \right)^{*} \right\}}{\Re \left\{ V_{n}^{\phi} \left( V_{0}^{\phi} \right)^{*} \right\}}.
%     \label{eqn:tanVkV0}
% \end{equation}
\begin{equation}
	\Re \left\{ V_{m}^{\phi} {\left( V_{n}^{\phi} \right)}^{*} \right\}
    \tan \left( \theta_{mn}^{\phi} \right)
    =
    \Im \left\{ V_{m}^{\phi} {\left( V_{n}^{\phi} \right)}^{*} \right\}
\end{equation}

\noindent The real and imaginary parts of $V_{mn}^{\phi}$ are defined as:
\begin{align}
    \Re \left\{ V_{m}^{\phi} {\left( V_{n}^{\phi} \right)}^{*} \right\}
    & = 
    \frac{1}{2} \left[ V_{m}^{\phi} {\left( V_{n}^{\phi} \right)}^{*} + V_{n}^{\phi} {\left( V_{m}^{\phi} \right)}^{*} \right] \nonumber \\
%     & =
%     \frac{1}{2} \left[ \Tr \left( \Phi_{V,mn}^{\phi} \mathbf{V} \right) + \Tr \left( \Phi_{V,nm}^{\phi} \mathbf{V} \right) \right] \\
    & =
    \frac{1}{2} \Tr \left( \left( \Phi_{V,mn}^{\phi} + \Phi_{V,nm}^{\phi} \right) \mathbf{V} \right) \\
	\Im \left\{ V_{m}^{\phi} {\left( V_{n}^{\phi} \right)}^{*} \right\}
    & =
    \frac{1}{j2} \left[ V_{m}^{\phi} {\left( V_{n}^{\phi} \right)}^{*} - V_{n}^{\phi} {\left( V_{m}^{\phi} \right)}^{*} \right] \nonumber \\
%     & =
%     \frac{1}{j2} \left[ \Tr \left( \Phi_{V,mn}^{\phi} \mathbf{V} \right) - \Tr \left( \Phi_{V,nm}^{\phi} \mathbf{V} \right) \right] \\
    & =
    \frac{1}{j2} \Tr \left( \left( \Phi_{V,mn}^{\phi} - \Phi_{V,nm}^{\phi} \right) \mathbf{V} \right) \qq ,
\end{align}

\noindent where $\Phi_{V,mn}^{\phi} = \overline{e}_{n}^{\phi} {\left( \overline{e}_{m}^{\phi} \right)}^{T}$ and $\Phi_{V,nm}^{\phi} = \overline{e}_{m}^{\phi} {\left( \overline{e}_{n}^{\phi} \right)}^{T}$ using the same convention for $\overline{e}_{n}^{\phi}$ as in \cite{dall2013distributed}. With some matrix algebra, we obtain equality constraints for the phase angle:
% \begin{align*}
% 	& \Tr \left( \left( \Phi_{n0}^{\phi} + \Phi_{0n}^{\phi} \right) X \right)
%     \tan \left( \theta_{n}^{\phi} - \theta_{0}^{\phi} \right) = \ldots \nonumber \\
%     & \quad -j \Tr \left( \left( \Phi_{n0}^{\phi} - \Phi_{0n}^{\phi} \right) X \right),
% \end{align*}
% \noindent which can be restated:
\begin{gather}
     \Tr \left(\Phi_{\theta,n0}^{\phi} \mathbf{V} \right) = 0 \label{eqn:SDPangeq} \\
     \Phi_{\theta,n0}^{\phi} = \sin \left( \theta_{n}^{\phi} - \theta_{0}^{\phi} \right)
    \left( \Phi_{V,n0}^{\phi} + \Phi_{V,0n}^{\phi} \right) \ldots
    \nonumber \\
    \quad \quad \quad \quad
    +
    j \cos \left( \theta_{n}^{\phi} - \theta_{0}^{\phi} \right) 
    \left( \Phi_{V,n0}^{\phi} - \Phi_{V,0n}^{\phi} \right).
    \label{eqn:PhiVn0}
\end{gather}

On the interval $\left( -\pi, \pi \right)$, $a \le b \Rightarrow \tan (a) \le \tan (b)$. Using this, we can define bounds on voltage angle difference.

The nature of SDPs disallows incorporation of the L2 norm, thus we were unable to formulate \eqref{eqn:OPF1} as an SDP. However, it is possible to formulate the SDP with an L1 norm minimization. We write an example objective function for an OPF where one node has a voltage magnitude reference:
\begin{equation}
	\min_{\mathbf{V}} \sum_{\phi \in \{ a,b,c \}} \left| \Tr \left( \Phi_{V,n}^{\phi} \mathbf{V} \right) - \Upsilon_{n}^{\phi} \right|
\end{equation}

\noindent This can be extended to a problem with multiple nodes having magnitude references. Similarly, \eqref{eqn:SDPangeq} and \eqref{eqn:PhiVn0} can be used in the same manner for phase angle references.
